# Supplementary material for: Pailitao-MMSearch: Building Native E-Commerce Multimodal Search Foundation
Source: arXiv:2607.17499 source file (2026-09-02)
Supplement: Supplementary file 1 [file 7-appendix.tex]

% \section{Appendix}

% \subsection{Eval Prompts fpr SIF and LIF}\label{sec:eval_prompts}

% % \begin{promptbox}{Eval Prompts}
% % You are a professional expert in evaluating product recommendation relevance.

% % \#\# Task

% % The user has provided an image and a search text, based on which the system has recommended a product. Please evaluate the relevance of the recommended product to the user's query.

% % \#\# User Query

% % - User image: See Image 1
% % - User search text: \{query\_text\}

% % \#\# Recommended Product

% % - Recommended product image: See Image 2
% % - Recommended product title: \{item\_title\}

% % \#\# Scoring Criteria (0-3 points)

% % - **3 points (Perfect Match)**: The product highly aligns with the search intent, consistent with the user's needs in terms of category, style, functionality, etc.

% % - **2 points (Good Match)**: The product is generally relevant to the search intent, with the correct category and broadly meeting the user's needs

% % - **1 point (Partial Relevance)**: The product has some connection to the search intent, but has obvious discrepancies in category, style, functionality, etc.

% % - **0 points (Not Relevant)**: The product is unrelated to the search intent, with incorrect category or completely failing to meet the user's needs

% % Please return strictly in JSON format without any other content:

% % {"score": <integer from 0-3>, "reason": "<brief evaluation reasoning, within 20 words>"}

% % \end{promptbox}

% \begin{promptbox}{Eval Prompts}
% 你是一位专业的商品推荐相关性评估专家。

% \#\# 任务

% 用户提供了一张图片和一段搜索文本，系统据此推荐了一件商品。请评估推荐商品与用户查询的相关性。

% \#\# 用户查询

% - 用户图片：见图片1

% - 用户搜索文本：\{query\_text\}

% \#\# 推荐商品

% - 推荐商品图片：见图片2

% - 推荐商品标题：\{item\_title\}

% \#\# 评分标准（0-3分）

% - **3分（完美匹配）**：商品与搜索意图高度吻合，品类、风格、功能等均与用户需求一致

% - **2分（较好匹配）**：商品与搜索意图基本相关，品类正确且大体符合用户需求

% - **1分（一般相关）**：商品与搜索意图有一定关联，但在品类、风格、功能等方面存在明显偏差

% - **0分（不相关）**：商品与搜索意图无关，品类错误或完全不符合用户需求

% 请严格以JSON格式返回，不要包含其他内容：

% {{"score": <0-3的整数>, "reason": "<简短评估理由，20字以内>"}}
% \end{promptbox}
